# Supplementary material for: Calculating the five-loop QED contribution to the electron anomalous magnetic moment: Graphs without lepton loops
Source: arXiv:1909.08015 ancillary file (2019-11-11)
Supplement: Supplementary file 1 [file readme.pdf]

## Description of the supplemental materials

The supplemental materials consist of 31 text files. All these files can be opened in a text editor as well as in spreadsheets like Excel or LibreOffice Calc (all real numbers in these files can be immediately used for arithmetical calculations). Each file consists of several lines containing the same number of elements separated by Tab character. All real numbers use comma as a decimal separator. Some of them are printed in the exponential notation; for example,  $-8,619883\text{e-}022$  means  $-8.619883 \cdot 10^{-22}$ . There are the following types of files in the materials:

1. 27 files with the names of the form

`class_⟨K⟩_⟨M⟩_⟨N⟩_⟨CALCULATION⟩.txt`.

These files contain a detailed information about individual Feynman graph contributions for the gauge-invariant class  $(K, M, N)$ .  $\langle \text{CALCULATION} \rangle$  takes one of the following values: `calc1`, `calc2`, `aver`. The first two ones correspond to the calculations Calc 1 and Calc 2 (see the main paper for the detailed explanation); the last one corresponds to the statistically combined results of these two calculations. For example, `class_3_1_1_aver.txt` has the combined results for the class  $(3, 1, 1)$ . The first line of each file contains the line element names. The other lines have these elements.

- **Number** is the Feynman graph number. The numeration is united. Each graph has a number from 1 to 3213. Graphs that are obtained from each other by changing arrow directions are regarded as one.
- **Graph\_code** is the code of the graph of the form

$$p; s_1 * f_1; s_2 * f_2; \dots; s_L * f_L$$

where  $p$  is the number of the vertex that is incident to the external photon line,  $L = 5$  is the number of independent loops in the graph,  $s_j$  and  $f_j$  are the ends of the  $j$ -th internal photon line; the vertexes are enumerated from 1 to  $2L+1$  along the electron path,  $s_j < f_j$ ,  $s_1 < \dots < s_L$ . The graphs are ordered lexicographically, and we guarantee that the code of a graph is the lexicographically minimal one. For example, the code of the 4-loop graph from FIG. 1 is `3;1*8;2*7;4*5;6*9`.

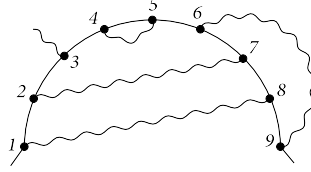

FIG 1. 4-loop Feynman graph: example

- **Contribution** is the contribution of this graph to  $A_1^{(10)}$ . All needed coefficients are contained in the values. Thus, the final values can be obtained simply by summation of the individual contributions.
- **sigma\_up, sigma\_down**:  $\sigma_{\uparrow}, \sigma_{\downarrow}$  for this graph and calculation.
- **N\_total** is the total number of Monte Carlo samples for the given graph and calculation.
- **N\_EIA\_fail** is the number of Monte Carlo samples for which the Eliminated Interval Arithmetic failed.
- **N\_IA\_fail** is the number of Monte Carlo samples for which the direct double-precision interval arithmetic failed.
- **N\_128\_fail** is the number of Monte Carlo samples for which the interval arithmetic with numbers of 128-bit mantissa failed.
- **N\_192\_fail** is the number of Monte Carlo samples for which the interval arithmetic with numbers of 192-bit mantissa failed.
- **N\_all\_fail** is the number of Monte Carlo samples for which the calculations with all precisions failed, including the interval arithmetic with numbers of 256-bit mantissa; the contribution of that points is assumed to be equal 0.
- **N\_double\_fail** is the number of Monte Carlo samples for which the machine double precision was not enough for storing the probability density.
- **Contr\_EIA\_fail** the contribution of the Monte Carlo samples for which the Eliminated Interval Arithmetic failed.
- **Contr\_IA\_fail** the contribution of the Monte Carlo samples for which direct double-precision interval arithmetic failed.
- **Contr\_128\_fail** the contribution of the Monte Carlo samples for which the interval arithmetic with numbers of 128-bit mantissa failed.

- **Contr\_192\_fail** the contribution of the Monte Carlo samples for which the interval arithmetic with numbers of 192-bit mantissa failed.
- **Contr\_double\_fail** the contribution of the Monte Carlo samples for which the machine double precision was not enough for storing the probability density.
- **Integral\_of\_abs** is the value of

$$\int |f(z_1, \dots, z_n)| \delta(z_1 + \dots + z_n - 1) d\mathbf{z},$$

where  $f(\mathbf{z})$  is the Feynman-parametric integrand for obtaining the contribution of the given graph to  $A_1^{(10)}$  with the needed coefficient included; the original contribution equals

$$\int f(\mathbf{z}) \delta(z_1 + \dots + z_n - 1) d\mathbf{z}.$$

- **Calc\_time** is the calculation time, GPU-sec.

2. 3 files with the names of the form

**sets\_for\_comparison\_<CALCULATION>.txt**

These files contain 807 sets of Feynman graphs for comparison with the direct subtraction on the mass shell in Feynman gauge and the contributions of these sets. These sets do not intersect and cover the whole set. Each set is contained in some gauge-invariant class  $(k, m, n)$ . **<CALCULATION>** takes one of the values **calc1**, **calc2**, **aver**. The files contain 4 columns:

- **Set**. Each set is represented as a sequence of Feynman graph numbers that are separated by a semicolon. The numeration is the same as in the files with individual contributions. The split into sets is the same in all three files.
- **Contribution**, **sigma\_up**, **sigma\_down** have the same meaning as in the files with individual contributions. These values are redundant and are added only for convenience. They can be obtained by summation and by using the formulas

$$\sigma_{\uparrow} = \sqrt{\sum_j (\sigma_{\uparrow,j})^2}, \quad \sigma_{\downarrow} = \sqrt{\sum_j (\sigma_{\downarrow,j})^2}$$

from the individual values.

3. 1 file

`total_numeration.txt`

This file with the correspondence between graph numbers and graph codes is redundant and is added for convenience.
